# Supplementary material for: The Price of Differential Privacy For Online Learning
Source: arXiv:1701.07953 source file (2017-06-13)
Supplement: Supplementary file 1 [file FTPLLemma.tex]

\section{FTPL for {\em Expert Advice} with $\Gamma(\eta, k)$ Noise}

\begin{lemma}
	Consider the online game $\{l_1, \ldots l_t\}$. Consider probability vectors $\{p_t\} \in \Delta_n$ defined as
	\[ p_t(i) = \pr{\argmin_{x \in \Delta_n} \left((\lsum{1}{t} + Z)\cdot x \right)  = e_i}\] 
	where $Z \sim \Gamma(\eta, k)$. Further we have that let $i_t$ be a random index sampled such that $\pr{i_t = i} = p_t(i)$ then the expected regret 
	\[\av{Regret} \defeq \av{ \sum_{t = 1}^{T} l_t(i_t) - min_{i \in [n]} \sum_{t = 1}^{T} l_t(i)} \leq \frac{k\log(n)}{\eta} + \sum_{t=1}^{T} \sum_{i = 1}^{n} \eta(p_t(i) l_t(i)^2)\]

	\na{The above might not be the correct precise expression. Will fix it when I get the right expression}  
\end{lemma}

\begin{proof}
	This proof follows the same steps as the proof from \cite{BartokNeu}. We will as is standard consider the the distribution if it knew the loss at time $t$ in advance in particular define 
	\[ \tilde{p}_t(i) = \pr{\argmin_{x \in \Delta_n} \left((\lsum{1}{t} + \tilde{Z})\cdot x \right)  = e_i} \]
	where $\tilde{Z}$ is $\sim \Gamma(\eta, k)$. We will first show a 'no' regret bound for an algorithm that plays according to $\tilde{p}_t$  

	The following lemma follows directly from Lemma 7 of \cite{BartokNeu}
	\begin{lemma} Lemma 7]
	\label{lemma:sub_lemma1}
		For any $i \in [n]$ we have that 
		\[\sum_{t=1}^{T} \sum_{j \in [n]} \tilde{p}_t(i)\left( l_t(j) - l_t(i)\right) \leq E_{\tilde{Z}} \left[\sum_{j \in [n]} \tilde{p}_1(j)(\tilde{Z}(j) - \tilde{Z}(i)) \right] \leq \frac{k \log(n)}{\eta}\] 
		
	\end{lemma}

	The first inequality of the lemma follows in a very standard fashion from the Follow the leader/ Be the leader lemma of \cite{kv}. Let 
	\[\tilde{i}_t \defeq \argmin_{x \in \Delta_n} \left(\lsum{1}{t} + \tilde{Z} \right)\]
	Then we have that for all $i$
	\[ \sum_{t=1}^{T} l_t(\tilde{i}_t) - \tilde{Z}(\tilde{i}_t) \leq \sum_{t=1}^{T} l_t(i) - \tilde{Z}(i)\]
	Taking expectation over $\tilde{Z}$ and rearranging gives the first inequality of the lemma. The second part as follows 
	\begin{align*}
		E_{\tilde{Z}} \left[\sum_{j \in [n]} \tilde{p}_1(j)(\tilde{Z}(j) - \tilde{Z}(i)) \right] &= E_{\tilde{Z}} \left[ \max_{j \in [n]} \tilde{Z}(j)\right] - E_{\tilde{Z}}\left[\tilde{Z}(i) \right]\\
		& \leq \frac{k \log(n)}{\eta}
	\end{align*}
	where the inequality follows from the following simple fact 
	\begin{fact}
		Let $Z(i) \sim \Gamma[\eta, k]$ are $n$ i.i.d random variables then then 
		\[ E[\max_i \tilde{Z}(i)] \leq \frac{k \log(n)}{\eta}\]
	\end{fact}

	We will now relate the regret of $p_t$ with $\tilde{p}_t$ via a suitable modification of Lemma 8 in \cite{BartokNeu}

	\begin{lemma}
	\label{lemma:sub_lemma2}
	 	For all $t = 1, 2, \ldots T$, assume that $\forall i \;\; l_t(i) \geq 0$. Then
	 	\[ \sum_j \left( p_t(j) - \tilde{p}_t(j) \right) l_t(j) \leq \eta \sum_{j} p_t(j)l_t^2(j)\]  
	 \end{lemma}

	 \begin{proof}
	 	Fix an arbitrary $t$ and $i' \in [n]$, and define the sparse loss vector $l_{t,i'}^{-}$ which is such that $l_{t,i'}^-(i) = l_t(i)$ if $i' = i$ and $0$ otherwise.

	 	Define \[p_{t}^{-}(i) \defeq \pr{\argmin_{x \in \Delta_n} \left((\lsum{1}{t} + l_{t,i}^- + \tilde{Z})\cdot x \right)  = e_i}\]
	 	And let $i_t^{-} \sim p_{t}^{-}$. The following lemma holds
	 	\begin{lemma}
	 		\[ p_{t}^{-} \leq \tilde{p}_t\] 	
	 	\end{lemma} 
	 	
	 	Also define the function
	 	\[ U(z) = \argmin_{x \in \Delta_n} \left( x^T \left( \lsum{1}{t} - z \right) \right)\]
	 	Let $f(z) = Pr_{\Gamma(\eta,k)}(z)$ we have that 
	 	\begin{align*}
	 		p_t(i) &= \int_{z \in \reals_+^d} 1_{\left(U(z) = u\right)} f(z) dz \\
	 		&\leq e^{\eta \|l_{t,i}^{-}\|_1} \int_{z \in \reals_+^d} 1_{\left(U(z) = u\right)} f(z + l_{t,i}^{-}) dz \\
	 		&= e^{\eta \|l_{t,i}^{-}\|_1} \int \int 
	 		\int_{z(j) \in [l_{t,i}(j), \infty]} 1_{\left(U(z - l_{t,i}^{-}) = u\right)} f(z) dz \\
	 		&\leq e^{\eta \|l_{t,i}^{-}\|_1} \int_{z \in \reals^d} 1_{\left(U(z - l_{t,i}^{-}) = u\right)} f(z) dz \\
	 		&\leq e^{\eta \|l_{t,i}^{-}\|_1} p_t^-(i) \\
	 		&\leq  e^{\eta \|l_{t,i}^{-}\|_1} \tilde{p}_t(i)\\
	 		&\leq  e^{\eta l_t(i)} \tilde{p}_t(i)
	 	\end{align*}

	 	Therefore we have that 
	 	\[ \tilde{p}_t(i) \geq p_t(i)e^{- \eta l_t(i)} \geq p_t(i)\left( 1 - \eta l_t(i)\right)\]

	 	The above equation holds for all $i$ and summing over all $i$ and reordering and we get the lemma. 

 	 \end{proof}
 	 The proof now follows from Lemma \ref{lemma:sub_lemma1} and \ref{lemma:sub_lemma2}
\end{proof}
