# Supplementary material for: The Price of Differential Privacy For Online Learning
Source: arXiv:1701.07953 source file (2017-06-13)
Supplement: Supplementary file 2 [file result.tex]

\section{Statement of the Result}
