# Supplementary material for: The Price of Differential Privacy For Online Learning
Source: arXiv:1701.07953 source file (2017-06-13)
Supplement: Supplementary file 3 [file sum_release.tex]

\subsection{Differentially Private Release of Sums}

\begin{lemma}[Differentially private release of sums]
	There exists a mechanism which takes as input vectors $\{v_1 \ldots v_t\}$ such that $\forall i \;\; \|v_i\|_{\infty} \leq L$ and outputs random vectors $\{\tilde{v}_1 \ldots \tilde{v}_t\}$ which satisfy the following conditions 
	\begin{itemize}
	 	\item \[\tilde{v}_i \sim v_{i \ldots i} + Z\]
		where $Z$ is a random vector distributed as $\Gamma(\eta, k)$ and the whole procedure 
		\item Moreover the whole procedure is Differentially Private with the following parameter 
		\[ poly(\frac{L}{\eta})\]
		\na{Note that it is very important that $L,\eta$ come with the same scale. As in we are screwed if the guarantee is $\frac{L^2}{\eta}$ or something} 	 
	 \end{itemize}

\end{lemma}
