# Supplementary material for: The Price of Differential Privacy For Online Learning
Source: arXiv:1701.07953 source file (2017-06-13)
Supplement: Supplementary file 4 [file old-notes.tex]

\section{Key questions to answer -}
% \begin{itemize}
% 	\item Can we merge Abernethy's analysis with Differential Privacy. The initial motivation is that we should not need more per step noise than $\sqrt{\frac{p}{\epsilon}} + \sqrt{T}$ to ensure differential privacy and this should should get us the right corresponding regret of essentially the same thing. 

% 	\item In terms of Bandits - the following is a natural progression of questions
% 	\begin{enumerate}
% 		\item Improve the regret bound of $T^{3/4}$ to $\sqrt{T}$ for the experts setting. Here the idea should be that exploration should naturally give some output perturbation. Not clear whether that is sufficient
% 		\item Linear losses - General conveex sets $\sqrt{T}$ regret
% 		\item Strongly Convex losses - General convex sets $\sqrt{T}$ regret
% 	\end{enumerate}
% \end{itemize}

These are the results we should shoot for 

\begin{itemize}
\item \textbf{Full Information}
	\begin{itemize}
			\item \textbf{Linear Losses, Weak Adversary, Simplex} I am condifdent that we have the following bound
	\[ \E[Regret] = O\left(polylog(n) \left(\frac{1}{poly(\epsilon)} + \sqrt{T} \right)\right) \]
	Moreover I think we can get this bound with the Gaussian as well as the Exponential Noise
	\na{TODO: Write a proof of this result}
	This improves upon the result of Jain and Thakurta \cite{icml2014c1_jain14}
	%#TODO - Write a proof of this statement

	\item \textbf{Linear Losses, Weak Adversary, General Convex Bodies} I am mildly confident all of Abernethy's case analysis follows here similarly as above. It seems not possible to guarantee optimal dependence on (dimension/convex body) here.
	\na{TODO: Write this up soon too} 

	\item \textbf{Convex Losses (Lipschitz/Smooth/Strongly Convex), Weak Adversary} - This once again seems hard because FTPL does not easily fit here. To get these results you need to play the expected output of FTPL per round

	\item \textbf{Both Cases above with Adaptive Adversary} - Once again taking the expectation outside screws things over here and therefore this case is not clear  

	\na{Can we show lower bounds in the above cases? Maybe approaching the Adaptive adversary first would be interesting} 
	\end{itemize}

\item \textbf{Bandits}
	\begin{itemize}
	\item \textbf{Experts Setting - Weak Adversary, Linear Losses, Simplex, Outputing one expert}
	I think, Apriori since noise is not treated as regularization (and they treat is an adversarial addition), they seem to be getting $T^{3/4}$. So FTPL's banditrization might be able to fix this and give us the bounds we require. As a first step lets get $\frac{T^{0.5}}{poly(\epsilon)}$ and then lets aim to make it $\epsilon$ free. 
	\na{Karan - Please enlighten us here}

	\item \textbf{General Linear Bandits over Convex Domains}
	I think this is especially hard since we dont know an FTPL based algorithm here

	\item \textbf{General Convex Losses}
	Out of scope !! 
	\end{itemize}
\end{itemize}
